# Supplementary material for: Useful Open Call-by-Need
Source: arXiv:2107.06591 source file (2021-10-28)
Supplement: Supplementary file 3 [file Rewriting_open_evaluation_contexts.tex]

% !TEX root = ../../../main.tex

\begin{proof}
\hfill

\begin{enumerate}		
	\item By induction on the derivation of $\pctx \in \evctxp{\varset}$:
		\begin{itemize}
			\item
			\emph{Rule $\ruleEvcAx$}: Let $\pctx = \progentry{\hctx}{\emptyenv} \in \evctxp{\nv{\hctx}}$. By \reflemmap{Rewriting_term_contexts-opencbneed}{one} (Term contexts give needed variables), $\var \in \nv{\hctxp{\var}}$. Hence, $\var \in \nv{\pctxp{\var}} = \nv{\hctxp{\var}}$.
			
			\item 
			\emph{Rule $\ruleEvcGc$}: Let $\pctx \in \evctxp{\varset}$ be derived as follows
				$$
				\infer
					[\ruleEvcGc]
					{\appES{\pctxtwo}{\esub{\vartwo}{\tm}} \in \evctxp{\varset}}
					{\pctxtwo \in \evctxp{\varset}
					\quad
					\vartwo \notin \varset}
				$$
			where $\pctx = \appES{\pctxtwo}{\esub{\vartwo}{\tm}}$. By hypothesis, $\var \neq \vartwo$ and $\var \notin \dom{\pctxtwop{\var}}$. By \ih, $\var \in \nv{\pctxtwop{\var}}$. Case analysis on whether $\vartwo \in \nv{\pctxtwop{\var}}$:
				\begin{itemize}
					\item Let $\vartwo \notin \nv{\pctxtwop{\var}}$. The statement follows because then $\nv{\pctxp{\var}} = \nv{\pctxtwop{\var}}$.
					
					\item Let $\vartwo \in \nv{\pctxtwop{\var}}$. Since $\var \neq \vartwo$, then
						$$
						\var \in (\nv{\pctxtwop{\var}} \setminus \set{\vartwo}) \subseteq (\nv{\pctxtwop{\var}} \setminus \set{\vartwo}) \cup \nv{\tm} = \nv{\pctxp{\var}}
						$$

				\end{itemize}
			
			\item
			\emph{Rule $\ruleEvcInert$}: Let $\pctx \in \evctxp{\varset}$ be derived as follows
				$$
				\infer
					[\ruleEvcInert]
					{\appES{\pctxtwo}{\esub{\vartwo}{\itm}} \in \evctxp{(\varsettwo \setminus \set{\vartwo}) \cup \nv{\itm}}}
					{\pctxtwo \in \evctxp{\varsettwo}
					\quad
					\vartwo \in \varsettwo}
				$$
			where $\pctx = \appES{\pctxtwo}{\esub{\vartwo}{\itm}}$ and $\varset = (\varsettwo \setminus \set{\vartwo}) \cup \nv{\itm}$. By \ih, we have that $\var \in \nv{\pctxtwop{\var}}$. Case analysis on whether $\vartwo \in \nv{\pctxtwop{\var}}$:
				\begin{itemize}
					\item Let $\vartwo \notin \nv{\pctxtwop{\var}}$. The statement follows because then $\var \in \nv{\pctxtwop{\var}} = \nv{\pctxp{\var}}$.
					
					\item Let $\vartwo \in \nv{\pctxtwop{\var}}$. Since $\var \neq \vartwo$, then
						$$
							\var \in \nv{\pctxtwop{\var}} \setminus \set{\vartwo} \subseteq (\nv{\pctxtwop{\var}} \setminus \set{\vartwo}) \cup \nv{\itm} = \nv{\pctxp{\var}}
						$$
					
				\end{itemize}
			
			\item
			\emph{Rule $\ruleEvcHer$}: Let $\pctx \in \evctxp{\varset}$ be derived as follows:
				$$
				\infer
					[\ruleEvcHer]
					{\appES{\pctxtwop{\vartwo}}{\esub{\vartwo}{\hctx}} \in \evctxp{\varsettwo \cup \nv{\hctx}}}
					{\pctxtwo \in \evctxp{\varsettwo}
					\quad
					\vartwo \notin \varsettwo}
				$$
			where $\pctx = \appES{\pctxtwop{\vartwo}}{\esub{\vartwo}{\hctx}}$ and $\varset = \varsettwo \cup \nv{\hctx}$. By $\alpha$-conversion, we may safely assume that $\vartwo \notin \dom{\pctxtwo}$. By \ih, we have that $\vartwo \in \nv{\pctxtwop{\vartwo}}$. Moreover, \reflemmap{Rewriting_term_contexts-opencbneed}{one} (Term contexts give needed variables) gives that $\var \in \nv{\hctxp{\var}}$. Hence,
				\begin{center}
					$
					\begin{array}{rcl}
						\var \in \nv{\hctxp{\var}} 
						& \subseteq & (\nv{\pctxtwop{\vartwo}} \setminus \set{\vartwo}) \cup \nv{\hctxp{\var}} \\
						& = & \nv{(\appES{\pctxtwop{\vartwo}}{\esub{\vartwo}{\hctx}}) \ctxholep{\var}} \\
						& = & \nv{\pctxp{\var}}
					\end{array}
					$
				\end{center}
				
		\end{itemize}
		
		\item Let $\tm$ be a term. We proceed by induction on the derivation of $\pctx \in \evctxp{\varset}$:
		\begin{itemize}
			\item
			\emph{Rule $\ruleEvcAx$}: Let $\pctx = \progentry{\hctx}{\emptyenv} \in \evctxp{\nv{\hctx}}$, with $\var \in \nv{\hctx}$. By \reflemmap{Rewriting_term_contexts-opencbneed}{three} (Focusing term contexts on needed variables), there exists a term context $\hctx_{\tm}$ such that $\var \notin \nv{\hctx_{\tm}} \subset \nv{\hctx}$ and that $\hctx_{\tm} \ctxholep{\var} = \hctxp{\tm}$. Thus, the statement holds by defining $\pctx_{\tm} \defeq \progentry{\hctx_{\tm}}{\emptyenv}$.
			
			\item 
			\emph{Rule $\ruleEvcGc$}: Let $\pctx \in \evctxp{\varset}$ be derived as follows
				$$
				\infer
					[\ruleEvcGc]
					{\appES{\pctxtwo}{\esub{\vartwo}{\tmtwo}} \in \evctxp{\varset}}
					{\pctxtwo \in \evctxp{\varset}
					\quad
					\vartwo \notin \varset}
				$$
			where $\pctx = \appES{\pctxtwo}{\esub{\vartwo}{\tmtwo}}$. By \ih with respect to $\var$ and $\pctxtwo$, there exists $\pctxtwo_{\tm} \in \evctxp{\varset_{\tm}}$ such that $\var \notin \varset_{\tm} \subset \varset$ and $\pctxtwo_{\tm} \ctxholep{\var} = \pctxtwop{\tm}$. We may then derive $\pctx_{\tm} \in \evctxp{\varset_{\tm}}$ as follows
				$$
				\infer
					[\ruleEvcGc]
					{\appES{\pctxtwo_{\tm}}{\esub{\vartwo}{\tmtwo}} \in \evctxp{\varset_{\tm}}}
					{\pctxtwo_{\tm} \in \evctxp{\varset_{\tm}}
					\quad
					\vartwo \notin \varset_{\tm}}
				$$
			where $\pctx_{\tm} = \appES{\pctxtwo_{\tm}}{\esub{\vartwo}{\tmtwo}}$, noting that $\pctx_{\tm} \ctxholep{\var} =  \appES{(\pctxtwo_{\tm} \ctxholep{\var})}{\esub{\vartwo}{\tmtwo}}  = \appES{(\pctxtwop{\tm})}{\esub{\vartwo}{\tmtwo}} = \pctxp{\tm}$.
								
			\item
			\emph{Rule $\ruleEvcInert$}: Let $\pctx \in \evctxp{\varset}$ be derived as
				$$
				\infer
					[\ruleEvcInert]
					{\appES{\pctxtwo}{\esub{\vartwo}{\itm}} \in \evctxp{(\varsettwo \setminus \set{\vartwo}) \cup \nv{\itm}}}
					{\pctxtwo \in \evctxp{\varsettwo}
					\quad
					\vartwo \in \varsettwo}
				$$
			where $\pctx = \appES{\pctxtwo}{\esub{\vartwo}{\itm}}$ and $\varset = (\varsettwo \setminus \set{\vartwo}) \cup \nv{\itm} $. Case analysis on whether $\var \in (\varsettwo \setminus \set{\vartwo})$:
				\begin{itemize}
					\item Let $\var \in (\varsettwo \setminus \set{\vartwo})$. Note that then $\var \notin \vartwo$. By application of the \ih with respect to $\var$ and $\pctxtwo$, there exists $\pctxtwo_{\tm} \in \evctxp{\varsettwo_{\tm}}$ such that $\var \notin \varsettwo_{\tm} \subset \varsettwo$ and $\pctxtwo_{\tm} \ctxholep{\var} = \pctxtwop{\tm}$. Now, if $\vartwo \notin \varsettwo_{\tm}$, then the statement holds by deriving $\pctx_{\tm}$ as follows
						$$
						\infer
							[\ruleEvcGc]
							{\appES{\pctxtwo_{\tm}}{\esub{\vartwo}{\itm}} \in \evctxp{\varsettwo_{\tm}}}
							{\pctxtwo_{\tm} \in \evctxp{\varsettwo_{\tm}}
							\quad
							\vartwo \notin \varsettwo_{\tm}}
						$$
					where $\pctx_{\tm} = \appES{\pctxtwo_{\tm}}{\esub{\vartwo}{\itm}}$. If $\vartwo \in \varsettwo_{\tm}$ instead, we proceed by case analysis on whether $\var \in \nv{\itm}$:
						\begin{enumerate}
							\item Let $\var \notin \nv{\itm}$. The statement then holds by deriving $\pctx_{\tm}$ as follows
								$$
								\infer
									[\ruleEvcInert]
									{\appES{\pctxtwo_{\tm}}{\esub{\vartwo}{\itm}} \in \evctxp{(\varsettwo_{\tm} \setminus \set{\var}) \cup \nv{\itm}}}
									{\pctxtwo_{\tm} \in \evctxp{\varsettwo_{\tm}}
									\quad
									\vartwo \in \varsettwo_{\tm}}
								$$
							where $\pctx_{\tm} = \appES{\pctxtwo_{\tm}}{\esub{\vartwo}{\itm}}$. Thus, and since $\var \neq \vartwo$ and $\var \notin \varsettwo_{\tm}$, we have that 
								$$
								\var \notin \varsettwo_{\tm} \setminus \set{\vartwo} \subset \varsettwo \setminus \set{\vartwo} \subseteq (\varsettwo \setminus \set{\vartwo}) \cup \nv{\itm} = \varset
								$$

							\item Let $\var \in \nv{\itm}$. By application of the \ih with respect to $\vartwo$ and $\pctxtwo_{\tm}$, there exists $\pctxtwo_{\var} \in \evctxp{\varsettwo_{\var}}$ such that $\vartwo \notin \varsettwo_{\var} \subset \varsettwo_{\tm} \subset \varsettwo$, and that $\pctxtwo_{\var} \ctxholep{\vartwo} = \pctxtwo_{\tm} \ctxholep{\var} = \pctxtwop{\tm}$.
							
							Moreover, by \reflemmap{Rewriting_term_contexts-opencbneed}{two} (Focusing inert terms on needed variables), there exists a term context $\hctx_{\var}$ such that $\var \notin \nv{\hctx_{\var}} \subset \itm$ and that $\hctx_{\var} \ctxholep{\var} = \itm$. Thus, we may derive $\pctx_{\tm} \in \evctxp{\varset_{\tm}}$ 
								$$
								\infer
									[\ruleEvcHer]
									{\appES{\pctxtwo_{\var} \ctxholep{\vartwo}}{\esub{\vartwo}{\hctx_{\var}}} \in \evctxp{\varsettwo_{\var} \cup \nv{\hctx_{\var}}}}
									{\pctxtwo_{\var} \in \evctxp{\varsettwo_{\var}}
									\quad
									\vartwo \notin \varsettwo_{\var}}
								$$
							where $\pctx_{\tm} = \appES{\pctxtwo_{\var} \ctxholep{\vartwo}}{\esub{\vartwo}{\hctx_{\var}}}$ and $\varset_{\tm} = \varsettwo_{\var} \cup \nv{\hctx_{\var}}$.

						\end{enumerate}
					
					\item Let $\var \notin (\varsettwo \setminus \set{\vartwo})$. Since $\var \in \varset = (\varsettwo \setminus \set{\vartwo}) \cup \nv{\itm}$, then it must be that $\var \in \nv{\itm}$. By application of the \ih with respect to $\vartwo$ and $\pctxtwo$, there exists $\pctxtwo_{\tm} \in \evctxp{\varsettwo_{\tm}}$ such that $\vartwo \notin \varsettwo_{\tm} \subset \varsettwo$ and $\pctxtwo_{\tm} \ctxholep{\vartwo} = \pctxtwop{\tm}$. Moreover, by \reflemmap{Rewriting_term_contexts-opencbneed}{two} (Focusing inert terms on needed variables), there exists term context $\hctx_{\var}$ such that $\var \notin \nv{\hctx_{\var}} \subset \nv{\itm}$ and $\hctx_{\var} \ctxholep{\var} = \itm$. Thus, we may derive $\pctx_{\tm} \in \evctxp{\varset_{\tm}}$ as follows
						$$
						\infer
							[\ruleEvcHer]
							{\appES{\pctxtwo_{\vartwo} \ctxholep{\vartwo}}{\esub{\vartwo}{\hctx_{\var}}} \in \evctxp{\varsettwo_{\vartwo} \cup \nv{\hctx_{\var}}}}
							{\pctxtwo_{\vartwo} \in \evctxp{\varsettwo_{\vartwo}}
							\quad
							\vartwo \notin \varsettwo_{\vartwo}}
						$$
					where $\pctx_{\tm} = \appES{\pctxtwo_{\vartwo} \ctxholep{\vartwo}}{\esub{\vartwo}{\hctx_{\var}}}$, verifying in particular that
						$$
							\pctx_{\var} \ctxholep{\var} = \appES{(\pctxtwo_{\vartwo} \ctxholep{\vartwo})}{\esub{\vartwo}{\hctx_{\var} \ctxholep{\var}}} = \appES{\pctxtwop{\tm}}{\esub{\vartwo}{\itm}} = \pctxp{\tm}
						$$							
				\end{itemize}
				
			\item 
			\emph{Rule $\ruleEvcHer$}: Let $\pctx \in \evctxp{\varset}$ be derived as
				$$
				\infer
					[\ruleEvcHer]
					{\appES{\pctxtwop{\vartwo}}{\esub{\vartwo}{\hctx}} \in \evctxp{\varsettwo \cup \nv{\hctx}}}
					{\pctxtwo \in \evctxp{\varsettwo}
					\quad
					\vartwo \notin \varsettwo}
				$$
			where $\pctx = \appES{\pctxtwop{\vartwo}}{\esub{\vartwo}{\hctx}}$ and $\varset = \varsettwo \cup \nv{\hctx}$. We do case analysis on whether $\var \in \varsettwo$:
				\begin{itemize}
					\item Let $\var \in \varsettwo$. By application of the \ih with respect to $\var$ and $\pctxtwo$, there exists $\pctxtwo_{\vartwo} \in \evctxp{\varsettwo_{\vartwo}}$ such that $\var \notin \varsettwo_{\vartwo} \subset \varsettwo$ and $\pctxtwo_{\vartwo} \ctxholep{\var} = \pctxtwop{\vartwo}$. Since $\vartwo \notin \varsettwo \supset \varsettwo_{\var}$, we can then derive $\pctx_{\tm} \in \evctxp{\varset_{\tm}}$ as follows
						$$
						\infer
							[\ruleEvcGc]
							{\appES{\pctxtwo_{\vartwo}}{\esub{\vartwo}{\hctxp{\tm}}} \in \evctxp{\varsettwo_{\vartwo}}}
							{\pctxtwo_{\vartwo} \in \evctxp{\varsettwo_{\vartwo}}
							\quad
							\vartwo \notin \varsettwo_{\vartwo}}
						$$
					where $\pctx_{\tm} = \appES{\pctxtwo_{\vartwo}}{\esub{\vartwo}{\hctxp{\tm}}}$, verifying in particular that
						$$
							\pctx_{\tm} \ctxholep{\var} = \appES{(\pctxtwo_{\vartwo} \ctxholep{\var})}{\esub{\vartwo}{\hctxp{\tm}}} = \appES{(\pctxtwo \ctxholep{\vartwo})}{\esub{\vartwo}{\hctxp{\tm}}} = \pctxp{\tm}
						$$
				
					\item Let $\var \notin \varsettwo$. Since $\var \in \varset = \varsettwo \cup \nv{\hctx}$, then it must be that $\var \in \nv{\hctx}$. By \reflemmap{Rewriting_term_contexts-opencbneed}{three} (Focusing term contexts on needed variables), there exists term context $\hctx_{\tm}$ such that $\var \notin \nv{\hctx_{\tm}} \subset \nv{\hctx}$ and $\hctx_{\tm} \ctxholep{\var} = \hctxp{\tm}$. Thus, we can derive $\pctx_{\tm} \in \evctxp{\varset_{\tm}}$ as follows
						$$
						\infer
							[\ruleEvcHer]
							{\appES{\pctxtwop{\vartwo}}{\esub{\vartwo}{\hctx_{\tm}}} \in \evctxp{\varsettwo \cup \nv{\hctx_{\tm}}}}
							{\pctxtwo \in \evctxp{\varsettwo}
							\quad
							\vartwo \notin \varsettwo}
						$$
					where $\pctx_{\tm} = \appES{\pctxtwop{\vartwo}}{\esub{\vartwo}{\hctx_{\tm}}}$.
											
				\end{itemize}
			
		\end{itemize}

\end{enumerate}

\end{proof}
