# Supplementary material for: Useful Open Call-by-Need
Source: arXiv:2107.06591 source file (2021-10-28)
Supplement: Supplementary file 23 [file Determinism_of_opencbneed.tex]

% !TEX root = ../../../main.tex

\begin{proof}
Let $\prog, \progtwo$, and $\progthree$ be programs. We have to prove that if $\prog \toond \progtwo$ and $\prog \toond \progthree$, then $\progtwo = \progthree$.
 Let $\tm_{1}, \tm_{2}$ be terms, $\pctx_{1} \in \evctxp{\varset_{1}}$ and $\pctx_{2} \in \evctxp{\varset_{2}}$ be such that $\prog = \pctx_{1} \ctxholep{\tm_{1}} = \pctx_{2} \ctxholep{\tm_{2}}$. Let moreover $S \defeq \varset_{1} \, \cup \, \varset_{2}$, noting that $\tm_{1}$ is a $S$-reduction place of $\pctx_{1} \ctxholep{\tm_{1}}$ and $\tm_{2}$ is a reduction place of $S$-reduction place of $\pctx_{2} \ctxholep{\tm_{2}}$. By \refthm{Unique_decomposition_of_programs-opencbneed} (Unique decomposition of programs), $\pctx_{1} = \pctx_{2}$ and $\tm_{1} = \tm_{2}$. Therefore, $\progtwo = \progthree$.\qedhere

\end{proof}
