# Supplementary material for: Useful Open Call-by-Need
Source: arXiv:2107.06591 source file (2021-10-28)
Supplement: Supplementary file 27 [file Properties_of_generalized_variables.tex]

% !TEX root = ../../../main.TEX

\begin{proof}
We proceed by induction on the derivation of $\genVarpr{\var}{\prog}$:
	\begin{itemize}
		\item If $\prog = \progentry{\var}{\emptyenv}$ then the statement clearly follows.
		
		\item Let $\genVarpr{\var}{\prog}$ be derived as follows
			$$
			\infer
				[\ruleGenVarHer]
				{\genVarpr{\var}{\appES{\progtwo}{\esub{\vartwo}{\var}}}}
				{\genVarpr{\vartwo}{\progtwo}}
			$$
		By \ih on $\progtwo$, $\nv{\progtwo} = \unv{\progtwo} = \set{\vartwo}$, $\anv{\progtwo} = \emptyset$ and $\sizend{\progtwo} = 0$\erase{ and $\unf{\progtwo} = \vartwo$}. The statement follows easily. In particular, note that $\unf{\prog} = \unf{\progtwo} \isub{\vartwo}{\var} =_{\ih} \vartwo \isub{\vartwo}{\var} = \var$.
		
		\item Let $\genVarpr{\var}{\prog}$ be derived as follows
			$$
			\infer
				[\ruleGenVarGc]
				{\genVarpr{\var}{\appES{\progtwo}{\esub{\vartwo}{\tm}}}}
				{\genVarpr{\var}{\progtwo}
				\quad
				\vartwo \neq \var}
			$$
		By \ih on $\progtwo$, $\nv{\progtwo} = \unv{\progtwo} = \set{\var}$, $\anv{\progtwo} = \emptyset$ and $\sizend{\progtwo} = 0$\erase{ and $\unf{\progtwo} = \var$}. The statement follows easily. In particular, note that $\unf{\prog} = \unf{\progtwo} \isub{\vartwo}{\var} =_{\ih} \var \isub{\vartwo}{\var} = \var$.\qedhere
		
	\end{itemize}
	
\end{proof}
