# Supplementary material for: Useful Open Call-by-Need
Source: arXiv:2107.06591 source file (2021-10-28)
Supplement: Supplementary file 28 [file Properties_of_useful_abstraction_programs.tex]

% !TEX root = ../../../main.TEX

\begin{proof}
By induction on the derivation of $\ufabspr{\prog}$:
	\begin{itemize}
		\item The statement holds trivially if $\prog = \progentry{\val}{\emptyenv}$. Moreover, $\unf{\progentry{\val}{\emptyenv}} = \val$.
		
		\item Let $\ufabspr{\prog}$ be derived as
			$$
			\infer
				[\ruleAbsGenVar]
				{\ufabspr{\appES{\progtwo}{\esub{\var}{\val}}}}
				{\genVarpr{\var}{\progtwo}}
			$$
		with $\prog = \appES{\progtwo}{\esub{\var}{\val}}$. Note that $\nv{\appES{\progtwo}{\esub{\var}{\val}}}  = \nv{\val}$---by \reflemma{Properties_of_generalized_variables} (Properties of generalized variables)---and so $\nv\prog = \emptyset$. We also have $\sizend{\appES{\progtwo}{\esub{\var}{\val}}} = \sizend{\progtwo} + \sizend{\val} =_{\reflemmaeq{Properties_of_generalized_variables}}  \sizend{\val} = 0$. Moreover, $\unf{\appES{\progtwo}{\esub{\var}{\val}}} = \un\progtwo\isub\var\val =_{\reflemmaeq{Properties_of_generalized_variables}}  \var\isub\var\val = \val$ which is a value.
				
		\item Let $\ufabspr{\prog}$ be derived as
			$$
			\infer
				[\ruleGenVarGc]
				{\ufabspr{\appES{\progtwo}{\esub{\var}{\tm}}}}
				{\ufabspr{\progtwo}}
			$$
		with $\prog = \appES{\progtwo}{\esub{\var}{\tm}}$. It follows easily by the \ih\qedhere

	\end{itemize}

\end{proof}
